# Supplementary material for: Effects of Lifshitz transitions in ferromagnetic superconductors: the case of URhGe
Source: arXiv:1805.02949 ancillary file (2018-05-08)
Supplement: Supplementary file 1 [file SuppMat3.pdf]

# Supplementary materials for "Role of Fermi surface topological transitions in ferromagnetic superconductors: the case of URhGe"

Yury Sherkunov[1], Andrey V. Chubukov[2] and Joseph J. Betouras[1]
[1]Department of Physics and Centre for the Science of Materials, Loughborough University, Loughborough, LE11 3TU, United Kingdom and
[2]Department of Physics, University of Minnesota, Minneapolis, Minnesota 55455, USA
(Dated: May 8, 2018)

## EFFECTIVE MASS ENHANCEMENT

Here we present our analysis of the effective mass enhancement of fermions occupying bands 1 and 2 subject to Zeeman splitting.

We start with the derivation of expressions for the effective mass enhancement (5), (10) - (12) of the main text following [1, 2]. The retarded Green's function of interacting electrons occupying band $\{i,\sigma\}$ obeys the Dyson equation:

$$\mathfrak{G}^R_{i\sigma}(\mathbf{p},\omega)=\frac{1}{\omega-\epsilon_{i\sigma}(\mathbf{p})-\Sigma^R_{i\sigma}(\mathbf{p},\omega)}, \tag{1}$$

where $\Sigma^R_{i\sigma}(\mathbf{p},\omega)$ is the retarded self-energy and $\epsilon_{i\sigma}(\mathbf{p})$ is the bare fermion energy. Expanding $\Sigma^R_{i\sigma}$ around $\{p_{i\sigma F},\omega=0\}$, and making a usual assumption that it is a slowly varying function of momentum, one arrives at the Fermion energies with $m_i\to m^*_{i\sigma}$ and $p_{i\sigma F}\to p^*_{i\sigma F}$, where the renormalised effective mass $m^*_{i\sigma}$ is given by Eq. (5) of the main text, and the renormalised Fermi momentum is $p^{*2}_{i\sigma F}=p^2_{i\sigma F}-2m_iRe[\Sigma^R_{i\sigma}(p_{i\sigma F},0)]$.

To calculate the self-energy, we use the Matsubara technique and assume $T=0$. In RPA [1, 2], the self-energy is given by the sum $\Sigma_{i\sigma}(\mathbf{p}_{i\sigma F},i\omega)=\Sigma^L_{i\sigma}(\mathbf{p}_{i\sigma F},i\omega)+\Sigma^T_{i\sigma}(\mathbf{p}_{i\sigma F},i\omega)$, where the longitudinal (L) and transverse (T) components are given by the sums of Feynman diagrams shown in Fig. 3 (a) and (b) 0f the main text respectively. First, we concentrate on the intra-band processes and write the self-energy as

$$\Sigma^l_{i\sigma}(\mathbf{p}_{i\sigma F},i\omega)=\int\frac{d\xi d^3q}{(2\pi)^4}G_{i\sigma'}(\mathbf{p}_{i\sigma F}-\mathbf{q},i(\omega-\xi))V_l(\mathbf{q},i\xi), \tag{2}$$

where $\sigma'=\sigma$ ($\sigma'=-\sigma$) for $l=L$ ($l=T$) and $V_L$ and $V_T$ are given by Eqs. (8) and (9) of the main text.

Now, we need to perform an analytical continuation of the Matsubara self-energy to calculated the retarded one. Using the spectral theorem $f(i\omega)=\frac{1}{\pi}\int dz\frac{Im[f(z+i0)]}{z-i\omega}$, where $f(z+i0)$ is the function analytical in the upper half-plane of complex $z$, one can express Eq. (2) as

$$\Sigma^l_{i\sigma}(\mathbf{p}_{i\sigma F},i\omega)=\int\frac{d\xi d^3qdz}{\pi(2\pi)^4}\frac{Im[V_l(\mathbf{q},z+i0)]}{[i(\omega-\xi)-\epsilon_{i\sigma'}(\mathbf{p}_{i\sigma F}-\mathbf{q})]}\times\frac{1}{z-i\xi}. \tag{3}$$

After integration with respect to $\xi$, Eq. (3) can be cast as

$$\Sigma^l_{i\sigma}(\mathbf{p}_{i\sigma F},i\omega)=-\int\frac{d^3qdz}{\pi(2\pi)^3}\frac{Im[V_l(\mathbf{q},z+i0)]}{i\omega-\epsilon_{i\sigma'}(\mathbf{p}_{i\sigma F}-\mathbf{q})-z}\times[f(\epsilon_{i\sigma'}(\mathbf{p}_{i\sigma F}-\mathbf{q}))-1-n(z)], \tag{4}$$

where $f$ and $n$ are Fermi and Bose functions. The main contribution to the effective mass enhancement comes from the terms proportional to $f$ [1], thus we neglect bosonic contribution. After integration with respect to azimuthal component of $\mathbf{q}$, performing the analytic continuation by substitution $i\omega\to\omega+i0$ and integrating with respect to $z$, one finds [1]

$$\Sigma^{l,R}_{i\sigma}(\mathbf{p}_{i\sigma F},\omega)=-\int_0^\infty\frac{m_iqdq}{(2\pi)^2p_{i\sigma F}}\int_{\epsilon_-}^{\epsilon_+}d\epsilon V_l(\mathbf{q},\omega-\epsilon+i0)f(\epsilon), \tag{5}$$

where $\epsilon_\pm=\epsilon_{i\sigma'}(p_{i\sigma}\pm q)$. To find the contribution to the effective mass enhancement, we differentiate $\Sigma$ with respect to $\omega$ and perform integration by parts in Eq. (5) neglecting the end-point contributions [1]. This leads to

$$[\partial_\omega\Sigma^{l,R}_{i\sigma}(\mathbf{p}_{i\sigma F},\omega)]_{\omega=0}=-\frac{m_i}{(2\pi)^2p_{i\sigma F}}\int_0^\infty qdq\int_{\epsilon_-}^{\epsilon_+}d\epsilon V_l(\mathbf{q},-\epsilon+i0)\delta(\epsilon), \tag{6}$$

where the $\delta-$ function restricts the $q-$integral to $p_l\le q\le p_u$ with $p_l=max\{0,p_{i\sigma F}-p_{i\sigma'F}\}$ and $p_u=p_{i\sigma F}+p_{i\sigma'F}$. Substituting Eq. (6) into Eq. (5) of the main text, we arrive at Eq. (10) of the main text with $\lambda^{i\sigma}_L$ and $\lambda^{i\sigma}_T$ given by Eqs. (11) and (12) of the main text respectively.

To calculate the effective mass enhancement numerically, we used Eq. (3) of the main text to derive the susceptibilities

$$\chi^{jj\sigma\sigma'}_0(\mathbf{q},0)=\frac{m_j(p_{j\sigma F}+p_{j\sigma'F})[(p_{j\sigma F}-p_{j\sigma'F})^2+q^2]}{8\pi^2q^2}\left[1+\frac{[(p_{j\sigma F}-p_{j\sigma'F})^2-q^2]}{2(p_{j\sigma F}+p_{j\sigma'F})q}\frac{[(p_{j\sigma F}+p_{j\sigma'F})^2-q^2]}{(p_{j\sigma F}-p_{j\sigma'F})^2+q^2}\times\ln\left|\frac{p_{j\sigma F}+p_{j\sigma'F}-q}{p_{j\sigma F}+p_{j\sigma'F}+q}\right|\right] \tag{7}$$

and calculated numerically the integrals of Eqs. (11)-(12) of the main text. The results shown in Fig. 1 suggest strong enhancement of the effective mass in the vicinity of $H_R$ as a result of Stoner-like instability (see the

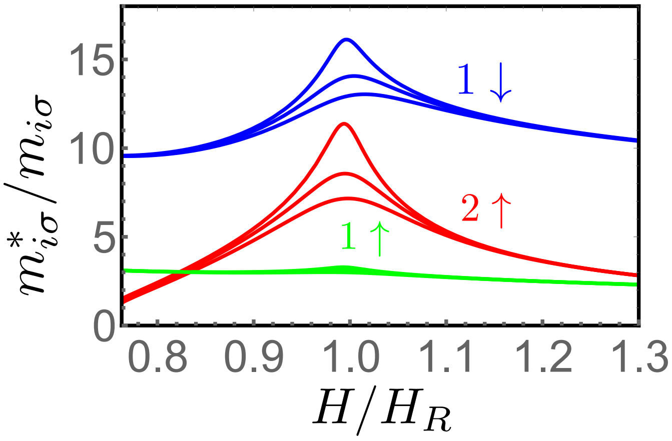


FIG. 1. Mass enhancement for the conduction electrons in the sub-bands 2 ↑ (red), 1 ↑ (green) and 1 ↓ (blue), as a function of magnetic field for $m_2 = 3m_1$, $U = 1.03/N(0)$ and $\mu_0/\epsilon^0_F = 1.5009;\ 1.5012;\ 1.5017$ (from top to bottom), where $N(0)$ and $\epsilon^0_F$ are the "paramagnetic" density of states and Fermi energy, $\epsilon^0_F = [3n(2\pi)^2/4]^{2/3}/(2m_1)$, and $n$ is the total electron density.

main text). The value of $m^*$ at $H_R$ demonstrates strong dependence on the inter-band energy shift $\mu_0$.

Now we take into account inter-band processes and calculate the self-energy given by

$$\Sigma^l_{i\sigma}(\mathbf{p}_{i\sigma F}, i\omega) = \int \frac{d\xi d^3q}{(2\pi)^4} G_{j\sigma'}(\mathbf{p}_{i\sigma F} - \mathbf{q}, i(\omega - \xi)) V^{ij}_l(\mathbf{q}, i\xi) \tag{8}$$

for $i \neq j$, where

$$V^{i,j,-\sigma}_L(\mathbf{q}, 0) = \frac{U^2 \chi^{ij,-\sigma,-\sigma}_0(\mathbf{q}, 0)}{1 - U^2 \chi^{ij,-\sigma,-\sigma}_0(\mathbf{q}, 0) \chi^{ij,\sigma,\sigma}_0(\mathbf{q}, 0)}, \tag{9}$$

$$V^{i,j,\sigma,-\sigma}_T(\mathbf{q}, 0) = \frac{U^3 [\chi^{ij,\sigma,-\sigma}_0(\mathbf{q}, 0)]^2}{1 - U \chi^{ij,\sigma,-\sigma}_0(\mathbf{q}, 0)} \tag{10}$$

for the longitudinal and transverse components respectively. The susceptibilities can be found from Eq. (3) of the main text:

$$\chi^{ij\sigma\sigma'}_0(\mathbf{q}, 0) = \frac{m_i m_j p_{i\sigma F}}{2\pi^2 (m_i - m_j)} \left[ 1 + \frac{(m_i - m_j) p_{i\sigma F}}{4 m_i q_0} \times \sum_{\alpha=\pm} (y^2_\alpha - 1) \ln \left| \frac{1 - y_\alpha}{1 + y_\alpha} \right| \right] + \{(i\sigma) \leftrightarrow (j\sigma')\}, \tag{11}$$

where $y_\pm = \{m_i q_0 \pm [m^2_j p^2_{i\sigma F} + m^2_i p^2_{j\sigma' F} - m_i m_j (p^2_{i\sigma F} + p^2_{j\sigma' F} - q^2_0)]^{1/2}\}/[(m_i - m_j) p_{i\sigma F}]$, and $\mathbf{q}_0 = \mathbf{q} + \mathbf{K}_0$. Eq. (11) peaks at $q_0 \to 0$, which corresponds to $q \sim K_0 \gg p_{i\sigma F}$. Following the derivation of Eq. (6), we find

$$[\partial_\omega \Sigma^{l,R}_{i\sigma}(\mathbf{p}_{i\sigma F}, \omega)]_{\omega=0} = -\frac{m_j}{(2\pi)^2 |\mathbf{p}_{i\sigma F} - \mathbf{K}_0|} \int_0^\infty q dq \int_{\epsilon'_-}^{\epsilon'_+} d\epsilon V^{ij}_l(\mathbf{q}, -\epsilon + i0) \delta(\epsilon), \tag{12}$$

where $\epsilon'_\pm = \epsilon_{j\sigma'}(p_{i\sigma} \pm q_0)$. Note, that Eq. (12) has large denominator $|\mathbf{p}_{i\sigma F} - \mathbf{K}_0|$ resulting from the shift between band 1 and band 2 in momentum space, $\mathbf{K}_0$. Thus, the contribution from inter-band processes can be important only at large transferred momenta, $q \sim K_0$, however, their contribution to the effective mass is suppressed due to large shifts between the two bands in the momentum space.

## SUPERCONDUCTIVE TRANSITION TEMPERATURE IN THE ABSENCE OF ORBITAL EFFECTS

Here we present the calculations of superconductive transition temperature $T_c$. First we neglect the orbital effects and use the strong coupling Eliashberg theory. At large $K_0$, inter-band scattering can be neglected, as shown above, and the transition temperature can be determined from linearised Eliashberg equations [3, 4] (see Eqs. (14) and (15) of the main text), where $V^{-\sigma}_L(q)$ and $V^{\sigma,-\sigma}_T(q)$ at finite temperatures are given by

$$V^{-\sigma}_L(q) = \frac{U^2 \chi^{-\sigma}_0(\mathbf{q}, \omega_n)}{1 - U^2 \chi^{-\sigma}_0(\mathbf{q}, \omega_n) \chi^{\sigma}_0(\mathbf{q}, \omega_n)}, \tag{13}$$

$$V^{\sigma,-\sigma}_T(q) = \frac{U^3 [\chi^{\sigma,-\sigma}_0(\mathbf{q}, \omega_n)]^2}{1 - U \chi^{\sigma,-\sigma}_0(\mathbf{q}, \omega_n)}, \tag{14}$$

with susceptibilities

$$\chi^{\sigma}_0(\mathbf{q}, \omega_n) = \sum_{i=1,2} \chi^{i,i,\sigma,\sigma}_0(\mathbf{q}, \omega_n),$$

$$\chi^{\sigma,-\sigma}_0(\mathbf{q}, \omega_n) = \sum_{i=1,2} \chi^{i,i,\sigma,-\sigma}_0(\mathbf{q}, \omega_n),$$

$$\chi^{i,i,\sigma,\sigma'}_0(\mathbf{q}, \omega_n) = T \sum_{l} G_{i,\sigma}(\mathbf{l}, \xi_m) G_{i,\sigma'}(\mathbf{l} + \mathbf{q}, \omega_n + \xi_m),$$

which can be calculated to yield

$$\chi^{i,i,\sigma,\sigma'}_0 = \frac{m_i}{32\pi^2 q^3} Re \left[ A + \sum_{\alpha=1,2} z^\alpha_+ z^\alpha_+ (\ln z^\alpha_- - \ln z^\alpha_+) \right], \tag{15}$$

where $A = -2q[(p_{i\sigma' F} - p_{i\sigma F})(z^1_+ + z^1_-) - 4 p_{i\sigma F} q^2]$, $z^1_\pm = p^2_{i\sigma F} - (p_{i\sigma' F} \pm q)^2 - 2i m_i w_n$, and $z^2_\pm = p^2_{i\sigma' F} - (p_{i\sigma F} \pm q)^2 + 2i m_i w_n$.

Using the Eliashberg approximation and integrating with respect to momenta, $\int d^3p ... = \int d\Omega \int d\epsilon N_{i\sigma}(0) ...$, where $\Omega$ is the solid angle, we can rewrite Eqs. (14) and (15) of the main text as

$$(1 - Z_{i\sigma}(p))\omega_n = -T\pi \sum_{\omega_{n'}} \int N_{i\sigma}(0) d\Omega_{\mathbf{p}'} \times V^{-\sigma}_z(p - p') sgn(\omega_{n'}), \tag{16}$$

$$|\omega_n Z_{i\sigma}(p)| \Phi_{i\sigma}(p) = -T\pi \sum_{\omega_{n'}} \int N_{i\sigma}(0) d\Omega_{\mathbf{p}'} \times V^{-\sigma}_W(p - p') \Phi_{i\sigma}(p'), \tag{17}$$

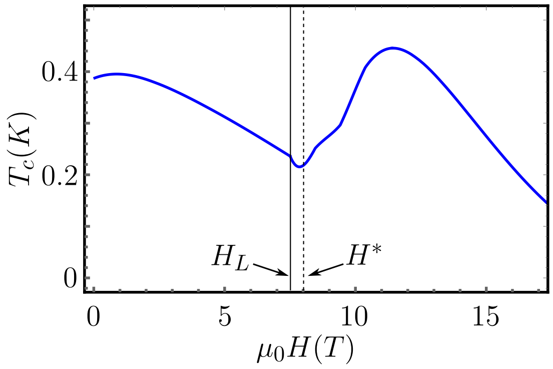


FIG. 2. $T_c$ without orbital effect. Same fitting parameters as in Fig. 1 of the main text. Vertical solid and dashed lines mark the magnetic field corresponding to the first Lifshitz transition $H_L$ and the change of the superconducting states from the majority ($H < H^*$) to the minority ($H > H^*$) bands respectively.

where we used a substitution $\Phi(p) = W(p)/|\omega_n Z(p)|$. Expanding $\Phi$ in spherical harmonics and retaining only the terms describing $p$-wave scattering, we can rewrite this set of equations as

$$\sum_{n'} \Big[ \lambda^{(1)}_{-\sigma}(\omega_n - \omega'_n) - \delta_{n,n'} \Big| \frac{\omega_n}{\pi T} + \sum_{l} \lambda^{(0)}_{-\sigma}(\omega_n - \omega_l) sgn(\omega_l) \Big| \Big] \Phi^1_{i\sigma}(\omega_{n'}) = 0, \quad (18)$$

which, using symmetry properties of $\lambda^{(0)}$ and $\lambda^{(1)}$ [4], can be cast as Eq. (16) of the main text. To calculate $T_c$, we convert Eqs. (16) and (17) of the main text to an eigenvalue problem by introducing a pair breaking parameter $\rho$ to the right-hand side:

$$\sum_{n \geq 0} K_{mn} \Phi^1_{i\sigma}(\omega_n) = \rho \Phi^1_{i\sigma}(\omega_m), \quad (19)$$

We solve Eq. (19) numerically truncating the sums at $N = 150$ and find the temperature, at which the maximal eigenvalue, $\rho$, is equal to zero. This temperature is equal to $T_c$. We checked the consistency of our results by increasing $N$ and checking its convergence. In calculating $T_c$ at high magnetic field, *i.e.* in the vicinity of $H_R$ we took into account only Zeeman splitting in the dispersion relations of electrons, as discussed in the main text. However, for small magnetic fields, for which ferromagnetism is strong, we also took into account the exchange splitting in the dispersion relations. The results are presented in Fig. 2. At small magnetic fields, band 2 does not cross the chemical potential and, thus, the superconducting states are formed in the majority band $1 \uparrow$. In this case, the transition temperature has maximum at small magnetic fields in agreement with [5]. Further increase of the magnetic field leads to the steady decrease of $T_c$, however, in the vicinity $\mu_0 H_L \approx 7.5T$ corresponding to the Lifshitz transition shown in Fig. 1 of the main text, where band 2 crosses the chemical potential, it reaches its minimum. We found that at $\mu_0 H \geq \mu_0 H^* \approx 8T$, the superconducting states are formed in minority band $1 \downarrow$, and $T_c$ starts to increase to reach its maximum at $\mu_0 H_R \approx 11.5T$.

To take into account the orbital effects, we follow [6] and calculates the transition temperature as $T_c^{orb}(H) = T_c(1 - H/H_c)$, where $H_c = \frac{20\pi k_B^2 T_c^2}{7\zeta(3) e\hbar v_F^2 \mu_0}$, as shown in Fig.1 of the main text.


[1] W. F. Brinkman and S. Engelsberg, Phys. Rev. **169**, 417 (1968).
[2] D. Fay and J. Appel, Phys. Rev. B **22**, 3173 (1980).
[3] P. B. Allen and R. C. Dynes, Phys. Rev. B **12**, 905 (1975).
[4] K. Levin and O. T. Valls, Phys. Rev. B **17**, 191 (1978).
[5] M. Kagan and A. Chubukov, JETP Lett **50**, 517 (1989).
[6] K. Scharnberg and R. A. Klemm, Phys. Rev. B **22**, 5233 (1980).
